# Supplementary material for: Specifying and Verifying Properties of Space - Extended Version
Source: arXiv:1406.6393 source file (2014-06-26)
Supplement: Supplementary file 1 [file appendix-b.tex]

\section{Some examples related to quasi-discreteness}

\begin{example}\label{exa:quasi-discrete-rational}
Existence of minimal neighbourhoods does not depend on finiteness of the space, and not even do they depend on existence of a ``closest element'' for each point. To see this, consider the rational numbers $\rats$, equipped with the relation $\leq$. Such a relation is reflexive and transitive, thus the closure space $(\rats,\closure_\leq)$ is topological and quasi-discrete.
\end{example}

\begin{example}\label{exa:quasi-discrete-not-topological}
Another example exhibiting minimal neighbourhoods in absence of closest elements is the following. Consider the rational numbers $\rats$ equipped with the relation $R = \{ (x,y) \mid |x - y| \leq 1 \}$, and let us look at the closure space $(\rats, \closure_R)$. $R$ is reflexive but not transitive, hence the obtained closure space is quasi-discrete but not topological. We have $\closure_R(A) = \{ x \in \rats \mid \exists a \in A . |a - x| \leq 1 \}$. Consider a point $x$. For $x$ to be included in $\interior(A)$, a set $A$ must include all the points whose distance from $x$ is less or equal than $1$, in other words, it must be true that $[x - 1, x + 1] \subseteq A$. To see this, suppose that there is $z \notin A$ such that $|z - x| \leq 1$. Then $x \in \closure_R(\{z\})$, thus since $\overline A = \overline A \cup \{z\}$, we have $x \in \closure_R(\overline A)$, and therefore $x \notin \interior(A) = \overline{\closure_R(\overline A)}$. The minimal neighbourhood is thus $N_x=[x-1,x+1]$. It is easily verified that $\interior(N_x)= \{ x \}$. In other words, each point $x$ has a minimal neighbourhood $N_x$, and there is no other point $y$ such that $N_x$ is a neighbourhood of $y$. However, there are infinitely many points belonging to $N_x$.
\end{example}

\begin{example}\label{exa:topological-not-quasi-discrete}
 An example of a topological closure space which is not quasi-discrete is the set of real numbers equipped with the Euclidean topology (the topology induced by arbitrary union and finite intersection of open intervals). To see that the space is not quasi-discrete, one applies \autoref{def:quasi-discrete-closure-space}. Consider an open interval $(x,y)$. We have $\closure((x,y)) = [x,y]$, but for each point $z$, we also have $\closure(z) = [z,z] = \{z\}$. Therefore $\bigcup_{ z \in (x,y) } \closure({z}) = \bigcup_{ z \in (x,y) } \{z\} = (x,y) \neq [x,y]$.
\end{example}

% \begin{example}
%  An example of a closure space which is neither topological nor quasi-discrete may be obtained by taking inspiration from \autoref{exa:quasi-discrete-not-topological} in the context of \autoref{exa:topological-not-quasi-discrete}. Consider the real numbers, equipped with the closure operator that associates to each non-empty subset $A$ the interval $[x-1,y+1]$, where $[x,y]$ is the least closed interval including $A$; we let $\closure(\emptyset) = \emptyset$ in order to fulfil the definition of closure.
%  %
%  Closure is not idempotent; consider e.g., the interval $(x,y)$, then we have $\closure((x,y)) = [x-1,y+1]$, whereas $\closure([x-1,y+1]) = [x-1,y+2]$. Also, the closure space is not quasi-discrete. To see this, observe that $\closure(\{z\}) = [z-1,z+1]$, that $\closure((x,y)) = [x-1,y+1]$ and finally that $\closure(\bigcup_{z \in (x,y)} \closure(\{z\}) = \bigcup_{z \in (x,y)} [z-1,z+1] = (x-1,y+1) \neq [x-1,y+1]$.
% \end{example}

\begin{example}
 The reader may think that quasi-discreteness is also related to the space having a smaller cardinality than that of the real numbers. This is not the case. To see this, just equip the real numbers with an arbitrary relation, e.g., the relation $\leq$, in a similar way to \autoref{exa:quasi-discrete-rational}. The obtained closure space is quasi-discrete.
\end{example}
